# Supplementary material for: Growth Mechanism and Origin of High $sp^3$ Content in Tetrahedral Amorphous Carbon
Source: arXiv:1804.07463 ancillary file (2018-04-20)
Supplement: Supplementary file 1 [file aC_growth_supplemental.pdf]

# Supplemental information: Growth mechanism and origin of high $sp^3$ content in tetrahedral amorphous carbon

Miguel A. Caro,[1,2,*] Volker L. Deringer,[3,4] Jari Koskinen,[5] Tomi Laurila,[1] and Gábor Csányi[3]

[1]*Department of Electrical Engineering and Automation, Aalto University, Espoo, Finland*
[2]*Department of Applied Physics, Aalto University, Espoo, Finland*
[3]*Engineering Laboratory, University of Cambridge, Trumpington Street, Cambridge CB2 1PZ, United Kingdom*
[4]*Department of Chemistry, University of Cambridge, Lensfield Road, Cambridge CB2 1EW, United Kingdom*
[5]*Department of Chemistry and Materials Science, Aalto University, Espoo, Finland*
(Dated: February 23, 2018)

This document contains miscellaneous supporting information pertaining our letter: "Growth mechanism and origin of high $sp^3$ content in tetrahedral amorphous carbon". We discuss i) the effect of substrate on deposition and substrate graphitization, ii) presence of a few 5-fold coordinated C atoms, iii) enlarged version of the middle and bottom panels of Fig. 5 of the letter with additional quantitative information.

## EFFECT OF SUBSTRATE THICKNESS ON THE RESULTS

To save CPU time, we chose a relatively thin $2 \times 1$ reconstructed diamond slab as substrate for production calculations, with 6 (111) monolayers and approximately 12 Å thickness. The total number of carbon atoms in the regular ("thin") substrate was 3240. We decided not to alter the dynamics of the bottom atoms so that the constraints would not introduce spurious effects on the growth characteristics due to, for instance, kinetic energy "bouncing off" a rigid wall of atoms. The graphitization of the lower surface occurs because the $2 \times 1$ (111) diamond surface reconstruction already contains $sp^2$ carbons and the $sp^3$ carbons which link those $sp^2$ carbons to the $sp^3$ diamond matrix present significantly longer out-of-plane bonds. This means that the barrier to transition between reconstructed surface and graphitic surface is relatively low. Once the transition occurs, the barrier for the reversed process is higher. The highly energetic impacting ions can activate the transition by transferring kinetic energy to the bottom atoms. To make sure that this is no artifact of the potential we simulated 475 deposition events on a significantly larger $2 \times 1$ (111) diamond substrate. Our simulation shows that with a thicker substrate the graphitization of the bottom layers does not occur (Fig. 1). Therefore, there is no artifact of the GAP potential. However, we decided not to run the production calculation of 8000 impacts with a thicker substrate since this increases the computational time substantially and does not provide any further insights once steady state growth sets in.

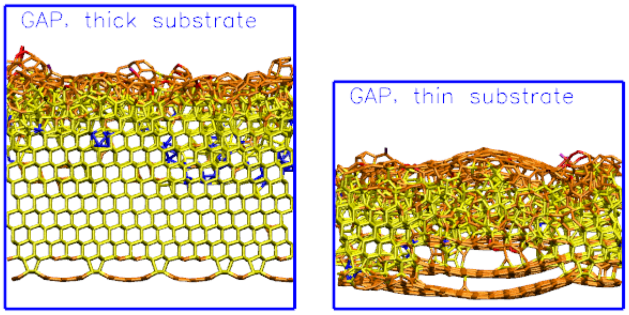


FIG. 1. Initial (111) diamond substrates and state of the substrates after circa 475 depositions.

## ORIGIN OF 5-FOLD COORDINATED C ATOMS

We can observe a small number of overcoordinated (5-fold coordinated) C atoms in our deposited films. While the number of 5-fold coordinated C atoms is very small, it is still worth it to trace down their origin and nature since 5-fold coordination is a coordination defect in C and thus energetically unfavorable. We find that 1.2% of deposited C atoms (that is, excluding the substrate atoms) in the last snapshot of the 60 eV deposition are 5-fold coordinated. Compare this to the 1.7% figure for 5-fold coordinated *incident* C atoms (top panel of Fig. 5 in our letter). This means that 29% of atoms which are deposited with 5-fold coordination move away from that configuration into a more stable one as the simulation

TABLE I. Average nearest-neighbor distances and standard deviations for the 5-fold coordinated atoms in the 60 eV film.

| Neighbor | Average distance (Å) | Standard deviation (Å) |
|---|---|---|
| 1st | 1.46 | 0.05 |
| 2nd | 1.50 | 0.04 |
| 3rd | 1.55 | 0.04 |
| 4th | 1.60 | 0.05 |
| 5th | 1.76 | 0.09 |

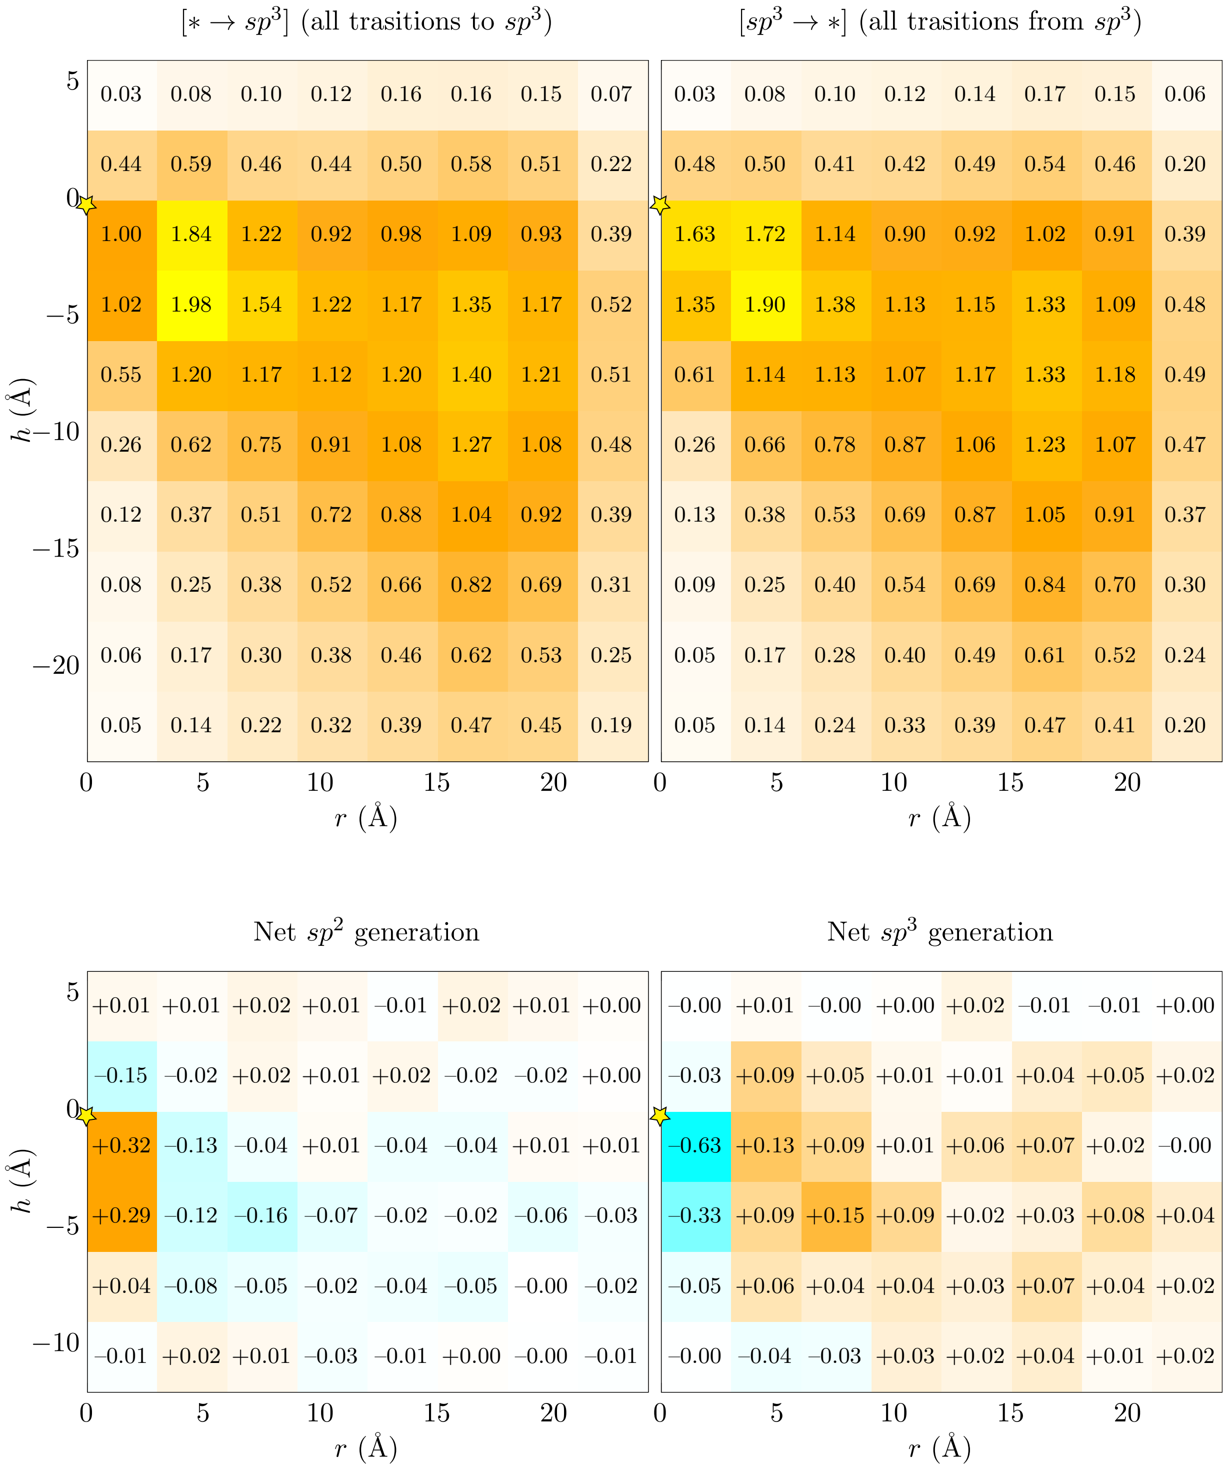


FIG. 2. Enlarged version of Fig. 5 from our letter. The numbers on the plot give the average number of bond rearrangement events *per impact* within each region.

progresses. To understand why the remaining 71% stay as 5-fold coordinated C, one needs to note that coordination is computed based on a nearest-neighbor cutoff distance. This is so since the GAP does not provide a representation of the electronic structure. Even within the context of DFT simulations, establishing $sp^2$ vs. $sp^3$ character is customarily also done based on a cutoff criterion, which tends to closely follow chemical character (as determined based on, e.g., local density of states analysis). We choose the cutoff distance as 1.9 Å, which is

the location of the minimum between the first and second peaks in the radial distribution function (see a more in-depth discussion in Ref [1]). A way to determine that 5-fold coordinated atoms are not an artifact of the potential is to look at the distance distribution of neighbors for those atoms: if there are 4 neighbors at distances close to that of diamond (around 1.5 Å) and another neighbor further apart (at, say, 1.8 Å), then this is a good indication that only 4 atoms will contribute to the bonding. We have looked in some detail at the distribution of nearest neighbors distances for 5-fold coordinated C atoms in the last snapshot of the 60 eV film. The results for average distances from closest to furthest neighbors and their standard deviations are given in Table I. As expected, the 5th neighbor is on average significantly further away than the other ones, and the spread of distances (standard deviation) is significantly larger. Furthermore, of those 5th-closest atoms, only 4.3% were less than 1.6 Å away. So, in summary, only 0.05% (4.3% of 1.2%) of all atoms in our 60 eV film had 5 neighbors all closer than 1.6 Å. We believe this gives a convincing argument that the small amount of detected 5-fold coordinated atoms is not an artifact of the a-C GAP potential and that it is not a cause for concern.

## GROWTH MECHANISM DETAIL

Figure 2 is an enlarged version of Fig. 5 from our letter, which allows to better appreciate the detailed features of the microscopic growth mechanism in ta-C.

* mcaroba@gmail.com

[1] M. A. Caro, R. Zoubkoff, O. Lopez-Acevedo, and T. Laurila, "Atomic and electronic structure of tetrahedral amorphous carbon surfaces from density functional theory: Properties and simulation strategies," Carbon **77**, 1168 (2014).
